# Supplementary material for: Compositor: Bottom-up Clustering and Compositing for Robust Part and Object Segmentation
Source: arXiv:2306.07404 source file (2023-11-30)
Supplement: Supplementary file 1 [file 07_supplementary.tex]

This document contains the supplementary materials for ``Compositor: Bottom-up Clustering and Compositing for Robust Part and Object Segmentation". It covers the detailed introduction and full results on Occluded-PartImageNet (\S\ref{sec:occ_partimagenet}), experimental results with stronger pixel decoder (\S\ref{sec:msde}), the correction of the errors in Tab. 3 and Tab. 4 and more ablation studies (\S\ref{sec:abla}), qualitative results on complicated scenes in Pascal-Part (\S\ref{sec:qual}) and error analysis for future work (\S\ref{sec:error}). 

\section{Results on Occluded-PartImageNet}
\label{sec:occ_partimagenet}
\textbf{Occluder categories.} To ensure that the categories of occluders do not have conflict with the categories in PartImageNet \cite{he2021partimagenet}. We sample 9 categories from COCO2014 \cite{lin2014microsoft} as occluders. To be specific, they are person, stop sign, handbag, umbrella, skateboard, potted plant, laptop, refrigerator and clock.

\textbf{Occlusion ratio.} We follow the pipeline of OccludedPASCAL3D+ \cite{wang2020robust} to superimposing occluders onto images of PartImageNet. The proposed Occluded-PartImageNet has 3 occlusion levels with different occlusion ratios of the foreground object. The occlusion ratio is computed as the number of occluded pixels on the foreground object mask dividing the number of object mask pixels. Note that since we can not strictly control the mask ratio of all images to be exactly the same number, we define the occlusion level based on a range of occluded ratios. Our three occlusion levels are defined as follow: Occluded-PartImageNet-v1: $20\% \sim 40\%$, Occluded-PartImageNet-v2: $40\% \sim 60\%$, Occluded-PartImageNet-v3: $60\% \sim 80\%$. The above numbers reflect different occluded ratios on the foreground object. Our Occluded-PartImageNet on all levels contains a roughly $0\% \sim 20\%$ occluded ratio on the background as well.

\begin{table}[]
\small
\centering
    \caption{Performance comparison on Occluded-PartImageNet-v2/v3. Numbers in brackets indicate performance drop compared to that on clean images.}
    \begin{tabular}{c|c|c|c}
        \multirow{2}{*}{\begin{tabular}[c]{@{}c@{}}occlusion \\ level\end{tabular}} & \multirow{2}{*}{method} & Part & Object \\ \cline{3-4} 
         &  & mIoU & mIoU \\ \hline
        \multirow{2}{*}{v2} & MaskFormer \cite{cheng2021per} & 44.02 \scriptsize{(-19.94\%)} & 49.81 \scriptsize{(-28.11\%)} \\
         & Compositor & \textbf{50.49} \scriptsize{(-16.19\%)} & \textbf{57.06} \scriptsize{(-21.89\%)} \\ \hline
        \multirow{2}{*}{v3} & MaskFormer \cite{cheng2021per} & 38.31 \scriptsize{(-25.65\%)} & 35.24 \scriptsize{(-42.68\%)} \\
         & Compositor & \textbf{44.41} \scriptsize{(-22.27\%)} & \textbf{43.83} \scriptsize{(-34.12\%)}
    \end{tabular}
    \label{tab:occ_supp}
\end{table}

\textbf{Performance on Occluded-PartImageNet}
We further report our Compositor's performance on the v2 and v3 levels of Occluded-PartImageNet to validate the robustness of Compositor against occlusion. Tab. \ref{tab:occ_supp} summarizes the performance comparison between Compositor and MaskFormer \cite{cheng2021per}. We observe that Compositor consistently presents much stronger robustness against occlusion by outperforming MaskFormer by around $6\%$ and $8\%$ in terms of part and object mIoU separately. Note that occlusion has a much more severe influence on object segmentation compared to part segmentation in both methods. This further indicates that learning low-level semantic information which is more robust against occlusion at first will help to improve the performance on high-level semantic tasks under occlusion if we could find a proper way to interact between them. We believe this points to a promising way to improve the model's ability to face out-of-distribution scenarios.

\begin{table*}[]
    \small
    \centering
    \caption{PartImageNet \textit{val} set results. mIoU, mACC on parts and objects are reported. MSDA represents the multi-scale deformable attention Transformer as introduced in \cite{zhu2020deformable}. $\dag$: Models on parts and objects are trained separately, $\ddag$: Models on parts and objects are trained jointly, $*$: Models on objects are trained with parts as deep supervision.}
    \begin{tabular}{l|c|c|cc|cc}
    \multirow{2}{*}{method} & \multirow{2}{*}{backbone} & \multirow{2}{*}{pixel decoder} & \multicolumn{2}{c|}{Part} & \multicolumn{2}{c}{Object} \\ \cline{4-7} 
     & & & mIoU & mACC & mIoU & mACC \\ \hline
    $\text{MaskFormer}^\dag$~\cite{cheng2021per} & ResNet-50~\cite{he2016deep} & MSDA \cite{zhu2020deformable} & 66.10 & 79.58 & 72.90 & 84.31 \\
    $\text{MaskFormer-Dual}^\ddag$ & ResNet-50~\cite{he2016deep} & MSDA \cite{zhu2020deformable} & 65.32 & 78.77 & 72.47 & 84.02 \\
    $\text{Compositor}^\ddag$ &
    ResNet-50~\cite{he2016deep} & MSDA \cite{zhu2020deformable} & \textbf{67.42} & \textbf{80.30} & \textbf{74.67} & \textbf{85.82} \\ \hline
    $\text{MaskFormer}^\dag$~\cite{cheng2021per} & Swin-T~\cite{liu2021swin} & MSDA \cite{zhu2020deformable} & 69.22 & 83.00 & 79.53 & 89.17 \\
    $\text{MaskFormer-Dual}^\ddag$ & Swin-T~\cite{liu2021swin} & MSDA \cite{zhu2020deformable} & 67.14 & 81.23 & 79.11 & 88.64 \\
    $\text{Compositor}^\ddag$ & Swin-T~\cite{liu2021swin} & MSDA \cite{zhu2020deformable} & \textbf{72.53} & \textbf{84.80} & \textbf{80.43} & \textbf{89.97}
    \end{tabular}
    \label{tab:deform_partimagenet}
\end{table*}

\begin{table*}[]
    \small
    \centering
    \caption{Pascal-Part \textit{val} set results. mIoU, mACC on parts and objects are reported. MSDA represents the multi-scale deformable attention Transformer as introduced in \cite{zhu2020deformable}. $\dag$: Models on parts and objects are trained separately, $\ddag$: Models on parts and objects are trained jointly, $*$: Models on objects are trained with parts as deep supervision.}
    \begin{tabular}{l|c|c|cc|cc}
    \multirow{2}{*}{method} & \multirow{2}{*}{backbone} & \multirow{2}{*}{pixel decoder} & \multicolumn{2}{c|}{Part} & \multicolumn{2}{c}{Object} \\ \cline{4-7} 
     & & & mIoU & mACC & mIoU & mACC \\ \hline
    $\text{MaskFormer}^\dag$~\cite{cheng2021per} & ResNet-50~\cite{he2016deep} & MSDA \cite{zhu2020deformable} & 51.41 & 62.88 & 76.15 & 86.92 \\
    $\text{MaskFormer-Dual}^\ddag$ & ResNet-50~\cite{he2016deep} & MSDA \cite{zhu2020deformable} & 50.05 & 61.26 & 75.87 & 86.47 \\
    $\text{Compositor}^\ddag$ &
    ResNet-50~\cite{he2016deep} & MSDA \cite{zhu2020deformable} & \textbf{52.76} & \textbf{64.04} & \textbf{77.90} & \textbf{88.46} \\ \hline
    $\text{MaskFormer}^\dag$~\cite{cheng2021per} & Swin-T~\cite{liu2021swin} & MSDA \cite{zhu2020deformable} & 57.29 & 70.06 & 82.02 & 91.86 \\
    $\text{MaskFormer-Dual}^\ddag$ & Swin-T~\cite{liu2021swin} & MSDA \cite{zhu2020deformable} & 56.27 & 69.41 & 81.55 & 91.43 \\
    $\text{Compositor}^\ddag$ & Swin-T~\cite{liu2021swin} & MSDA \cite{zhu2020deformable} & \textbf{57.90} & \textbf{70.79} & \textbf{83.31} & \textbf{92.64}
    \end{tabular}
    \label{tab:deform_pascal}
\end{table*}

\section{Experimental Results with Stronger Pixel Decoder}
\label{sec:msde}
To validate the generalizability of our Compositor in terms of the choice of pixel decoder, we also experiment with the heavy multi-scale deformable attention Transformer (MSDA) \cite{zhu2020deformable}. As can be observed from Tab. \ref{tab:deform_partimagenet} and Tab. \ref{tab:deform_pascal}, by equipping Compositor with the strong pixel decoder MSDA, the performance gets a huge improvement. We observe that such a strong pixel decoder brings more improvement to part segmentation compared to object segmentation. Note that our Compositor consistently outperforms either the MaskFormer specialized in single-task or the MaskFormer-Dual baseline by a non-trivial margin.

\section{Ablation Studies}
\label{sec:abla}
\textbf{Correction on Ablation Studies in Tab. 3 and Tab. 4}. We are sorry about the mistakes we made in Tab. 3 and Tab. 4 in the Experiments Section of the paper. The Object mIoU column is wrongly filled with numbers of the Part mACC metric in these two tables instead of the desired Object mIoU. We first correct this error and show the right results below:

\begin{center}
    \begin{minipage}{0.47\textwidth}
        \begin{minipage}[t]{0.48\textwidth}
            \centering
            \makeatletter\def\@captype{table}\makeatother
            \small
            \caption{Corrected ablation study on part and object loss ratio $\beta$ with Swin-T on Pascal-Part.}
            \label{tab:weight}
            \begin{tabular}{c|c|c}
                \multirow{2}{*}{$\beta$} & Part & Object \\ \cline{2-3} 
                 & mIoU & mIoU \\ \hline
                1/4 & 55.04 & 81.97 \\
                \rowcolor{Gray}
                1/3 & \textbf{55.36} & \textbf{82.65} \\
                1/2 & 54.86 & 82.16 \\
                1 & 53.38 & 82.03 \\
                2 & 51.41 & 81.74
            \end{tabular}
        \end{minipage}
        \begin{minipage}[t]{0.48\textwidth}
            \centering
            \makeatletter\def\@captype{table}\makeatother
            \small
            \caption{Corrected ablation study on numbers of queries (\ie, N/M) with Swin-T on Pascal-Part.}
            \label{tab:part_q}
            \begin{tabular}{c|c|c}
                \multirow{2}{*}{N/M} & Part & Object \\ \cline{2-3} 
                 & mIoU & mIoU \\ \hline
                15/40 & 54.47 & 81.74 \\
                15/50 & 54.68 & 82.03 \\
                \rowcolor{Gray}
                20/50 & \textbf{55.36} & \textbf{82.65} \\
                25/50 & 55.30 & 82.48 \\
                20/60 & 54.71 & 82.21
            \end{tabular}
      \end{minipage}
    \end{minipage}
\end{center}

\textbf{Additional Ablation Studies with ResNet-50}. To ensure the conclusion in our ablation studies is general to different backbones, we offer additional experimental results of these ablation studies with ResNet-50 as the backbone here. As can be observed from Tab. \ref{tab:supp_weight} and Tab. \ref{tab:supp_part_q}, the conclusion we made still holds here.

\begin{center}
    \begin{minipage}{0.47\textwidth}
        \begin{minipage}[t]{0.48\textwidth}
            \centering
            \makeatletter\def\@captype{table}\makeatother
            \small
            \caption{Ablation study on part and object loss ratio $\beta$ with ResNet-50 on Pascal-Part.}
            \label{tab:supp_weight}
            \begin{tabular}{c|c|c}
                \multirow{2}{*}{$\beta$} & Part & Object \\ \cline{2-3} 
                 & mIoU & mIoU \\ \hline
                1/4 & 48.97 & 76.44 \\
                \rowcolor{Gray}
                1/3 & \textbf{49.53} & \textbf{77.03} \\
                1/2 & 48.70 & 76.82 \\
                1 & 47.72 & 76.29 \\
                2 & 45.88 & 74.93
            \end{tabular}
        \end{minipage}
        \begin{minipage}[t]{0.48\textwidth}
            \centering
            \makeatletter\def\@captype{table}\makeatother
            \small
            \caption{Ablation study on numbers of queries (\ie, N/M) with ResNet-50 on Pascal-Part.}
            \label{tab:supp_part_q}
            \begin{tabular}{c|c|c}
                \multirow{2}{*}{N/M} & Part & Object \\ \cline{2-3} 
                 & mIoU & mIoU \\ \hline
                15/40 & 47.81 & 76.21 \\
                15/50 & 48.87 & 76.68 \\
                \rowcolor{Gray}
                20/50 & 49.53 & \textbf{77.03} \\
                25/50 & \textbf{49.72} & 76.66 \\
                20/60 & 49.23 & 76.64
            \end{tabular}
      \end{minipage}
    \end{minipage}
\end{center}

\section{Qualitative Results}
\label{sec:qual}
We show additional qualitative results on Pascal-Part \cite{chen2014detect} \textit{val} set here since the Pascal-Part dataset contains many complicated images with multiple different objects with different poses. As can be seen from Fig.\ref{fig:supp_vis}, our Compositor is able to handle such complicated scenarios by segmenting most of the parts accurately. Though our model still exhibits errors when different parts appear at the same location (\eg, row 2) and ignores some small parts at far position (\eg row 1), note that most of the errors are actually inner errors (\ie, the boundary between different parts within an object). This is inevitable since even the human annotations will be inconsistent in such scenarios and many of the model's predictions on boundary actually makes sense. This implies that the current evaluation metrics might underestimate the part segmentation model and a better metric for evaluating these algorithms is desired.

\begin{figure*}[t!]
    \small
    \centering
    \includegraphics[width=0.62\textwidth]{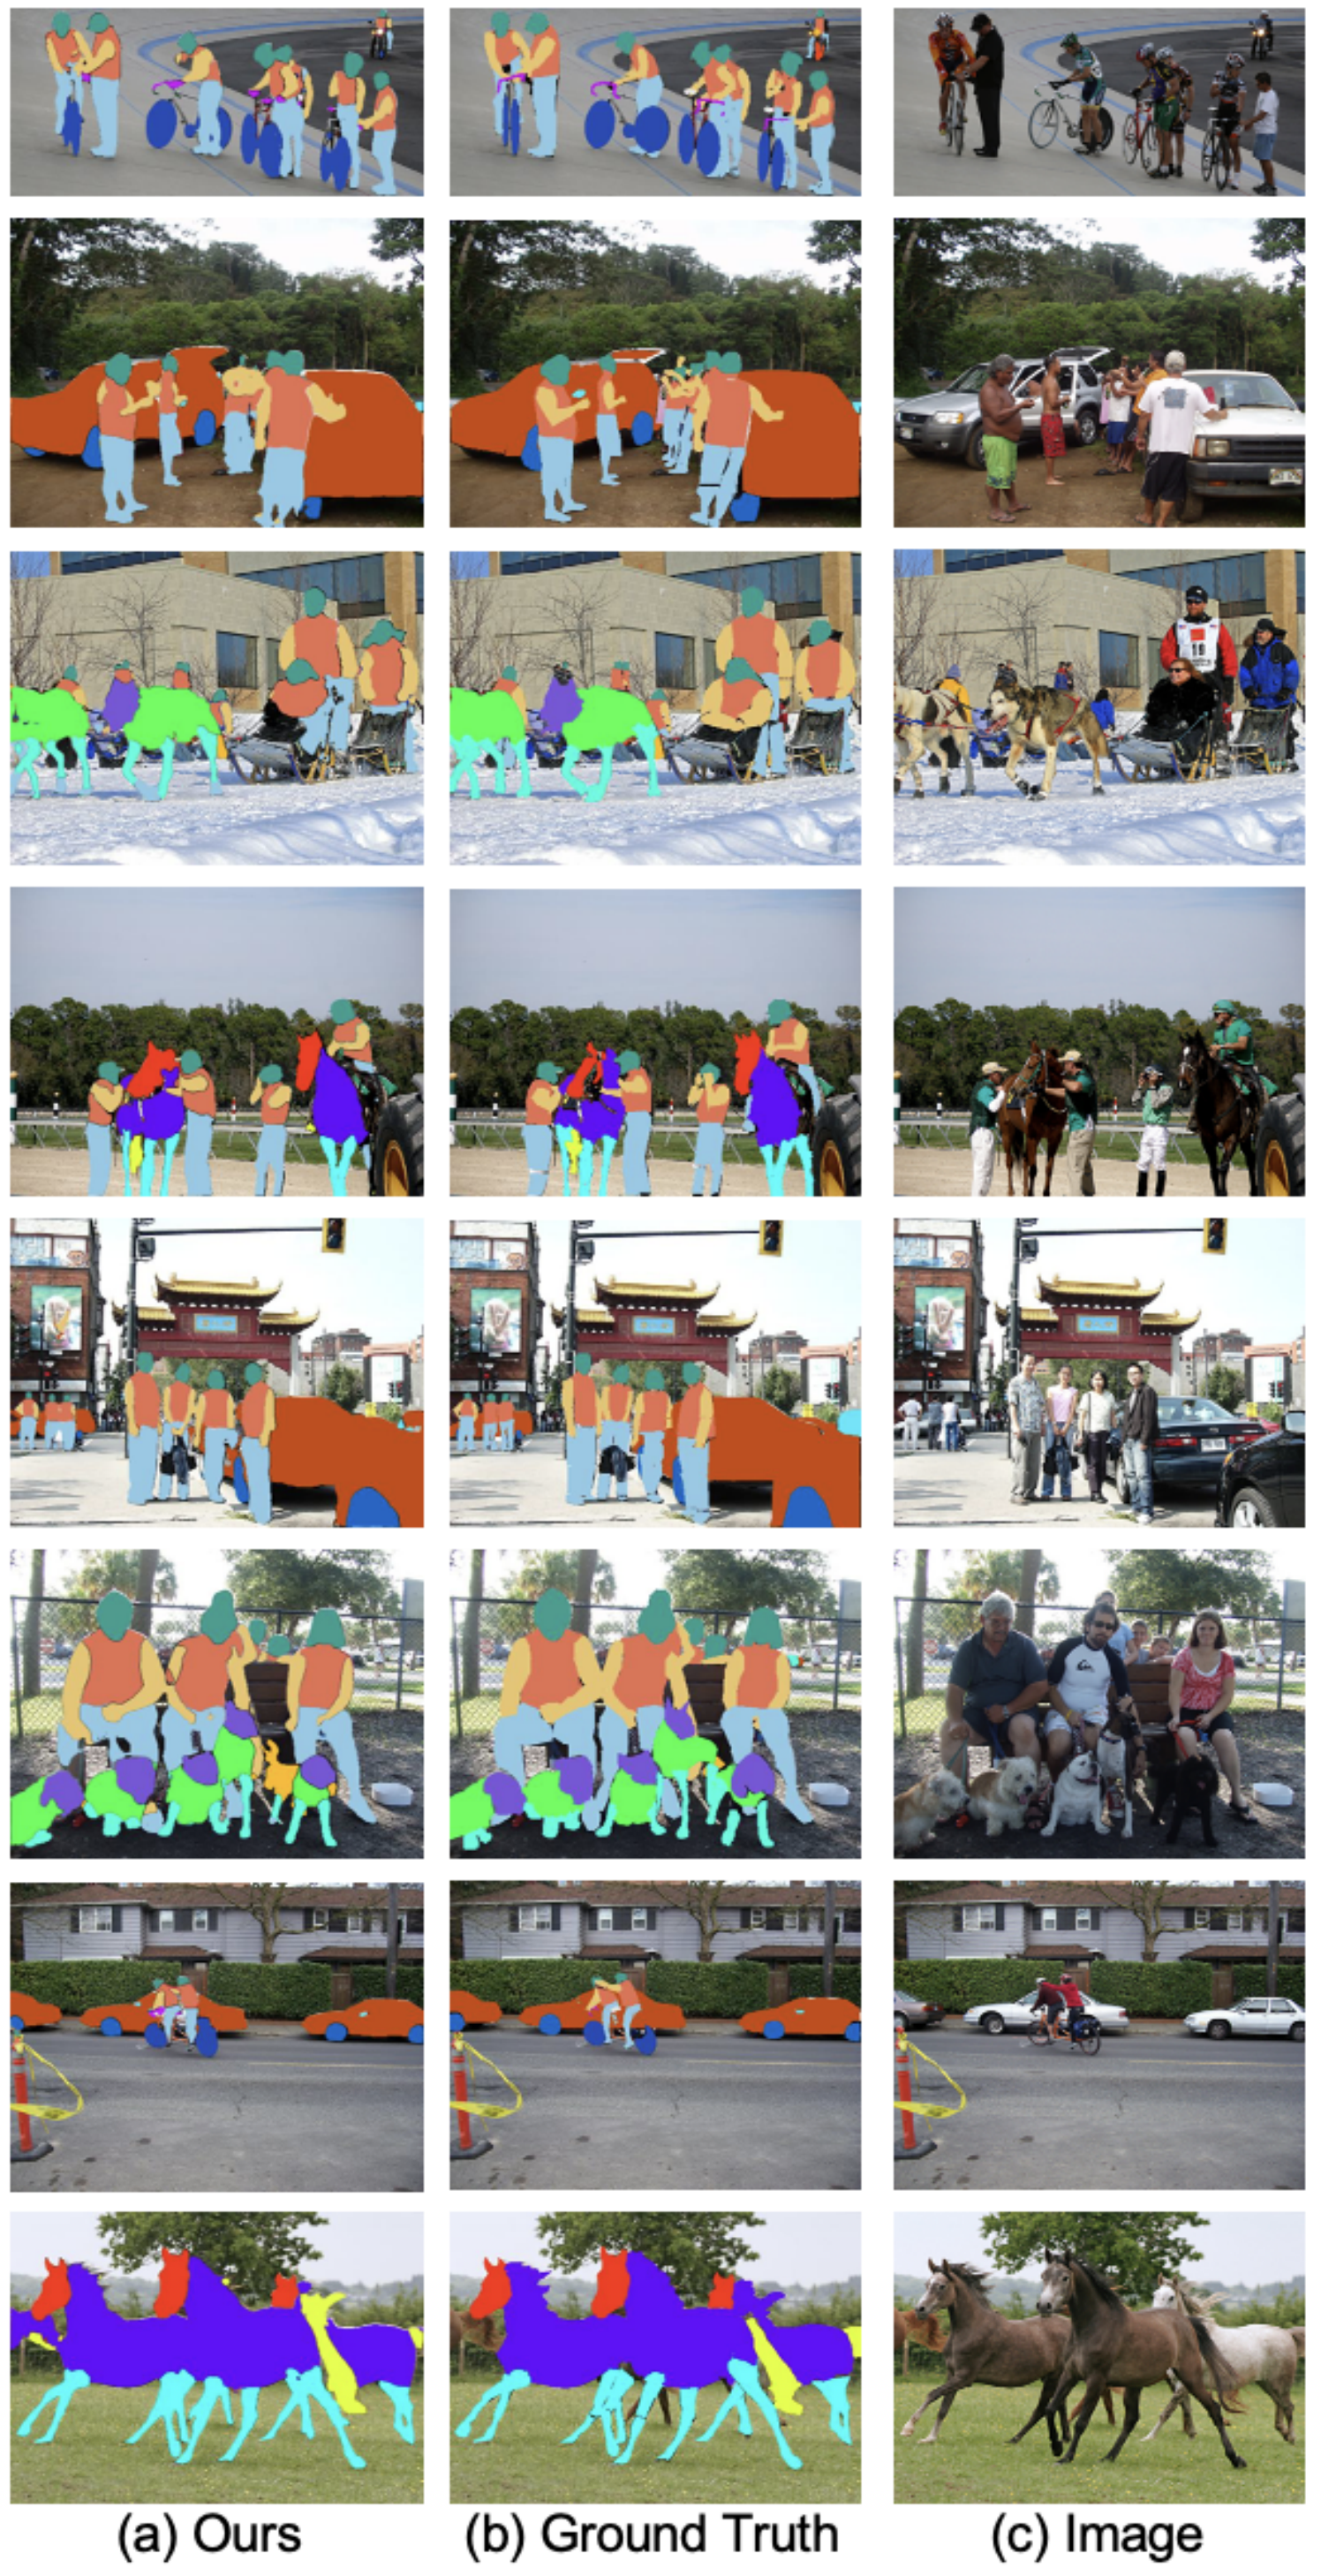}
    \caption{Qualitative results on Pascal-Part. Note how Compositor successfully segment parts accurately in these very complicated scenes.}
    \label{fig:supp_vis}
\end{figure*}

\begin{figure*}[t!]
    \small
    \centering
    \includegraphics[width=0.95\textwidth]{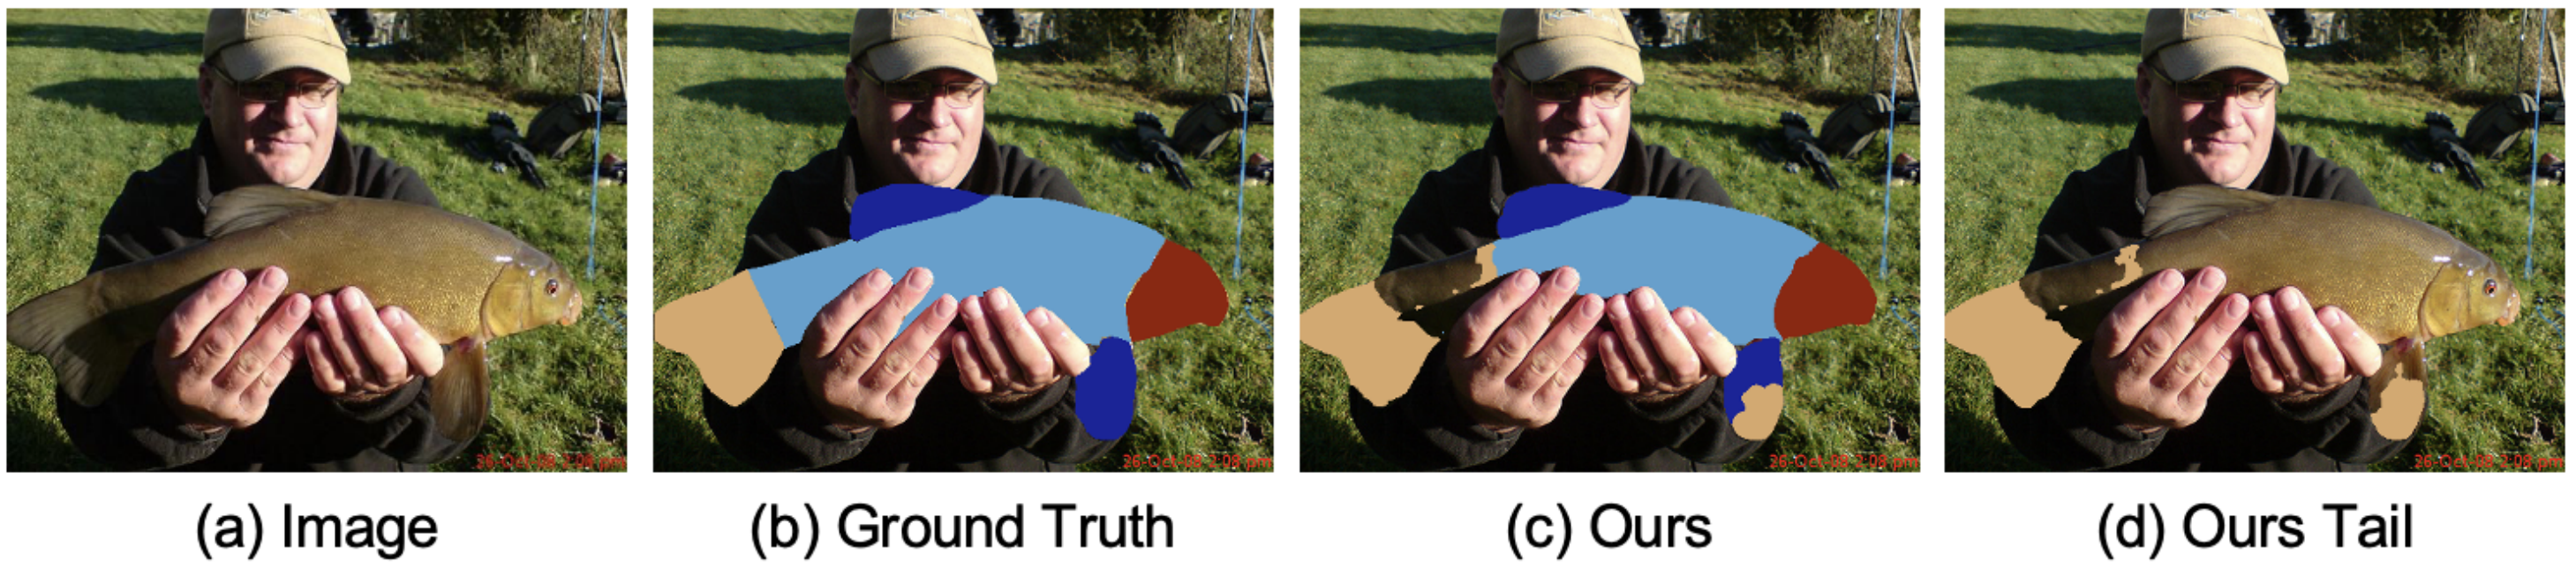}
    \caption{Example figure for error analysis.}
    \label{fig:supp_error}
\end{figure*}

\section{Error Analysis and Future Work}
\label{sec:error}
As introduced in the ``Error Analysis" subsection in the paper, we conduct a detailed analysis of our model from the perspective of part detection. Here we further take Fig.\ref{fig:supp_error} for example to illustrate how our model can be improved in the future. Despite the inner error (\ie, boundary between fish's body and fish's tail), the main error of this figure comes from the segmentation of the tail. The error on the fish's tail can be further divided into two parts: 1) The missing prediction at the location of the human's arm; 2) The false prediction at the location of the fish's fin. 

The first kind of error is harder to solve here since the color and texture of the clothes on the arm are very similar to those of the fish body. Such missing prediction might also be caused by the natural occlusion (\eg, putting the man's hands on the missing area) so it can not be simply fixed by post-processing such as requiring the parts to be connected. A well-trained model with a stronger backbone/pixel decoder might be able to solve such kind of problems. 

We mainly target at the second type of the error. Our result shows that in this wrongly classified area, the model also has a high probability to predict it as the correct label ``fin'' instead of the ``tail'' (corresponds to the Top-3 analysis in Tab. 6). The model is much less confident in predicting the ``tail'' label there compared to the prediction on the real tail region. We argue that such errors can be improved by introducing a better object model, probably containing pose or 3D information of the object. In such scenarios, the model will know that given the locations of other confidential predicted parts, the ``tail'' is impossible to appear there and can thus pick a prediction label either from the 2nd or the 3rd possible choices or from neighbors. We leave this interesting problem to future research.
